# Supplementary material for: Symmetry breaking in collective decision-making through higher-order interactions
Source: arXiv:2510.00853 ancillary file (2025-10-01)
Supplement: Supplementary file 1 [file supp.pdf]

# Supplemental Material for: Symmetry breaking in collective decision-making through higher-order interactions

David March-Pons,<sup>1,2,\*</sup> Romualdo Pastor-Satorras,<sup>1</sup> and M. Carmen Miguel<sup>2,3</sup>

<sup>1</sup>*Departament de Física, Universitat Politècnica de Catalunya, Campus Nord B4, 08034 Barcelona, Spain*

<sup>2</sup>*Departament de Física de la Matèria Condensada,  
Universitat de Barcelona, Martí i Franquès 1, 08028 Barcelona, Spain.*

<sup>3</sup>*Institute of Complex Systems (UBICS), Universitat de Barcelona, 08028 Barcelona, Spain*

## SUPPLEMENTAL FIGURES

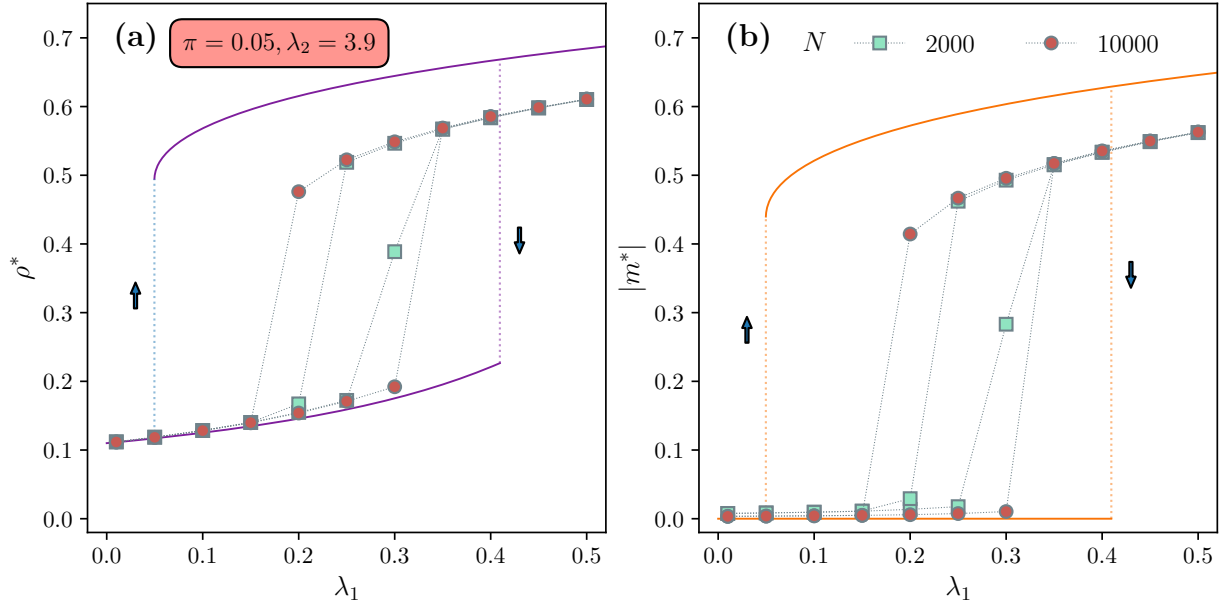

FIG. SF1: Size dependence of the hysteresis cycle for spontaneous adoption  $\pi = 0.05$  and group recruitment strength  $\lambda_2 = 3.9$ . (a), (b) show the stationary values of the active population  $\rho^*$  and the absolute consensus  $|m^*|$ , respectively. The results for system size  $N = 2000$  correspond to those presented in the main text, Figure 3 (b,c). Additionally, we include simulations with  $N = 1000$ , which show a slight increase in the hysteresis cycle's width, suggesting that this trend may continue for larger system sizes. Node degree and simplicial degree are  $\langle k \rangle = 20$  and  $\langle k_2 \rangle = 6$ .

\*Electronic address: [david.march@upc.edu](mailto:david.march@upc.edu)

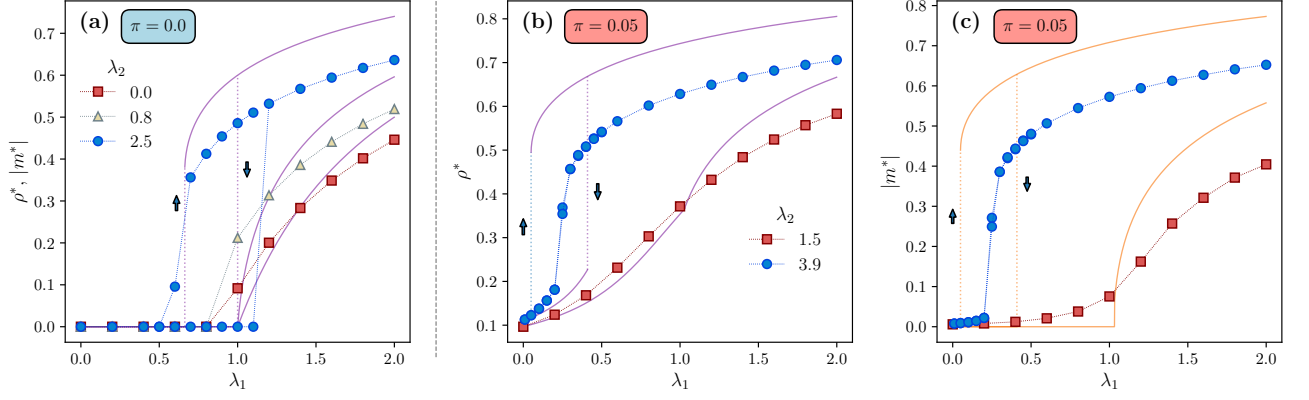

FIG. SF2: Simulations on a Random Simplicial Complex (RSC) with  $\langle k \rangle = 6$  and  $\langle k_2 \rangle = 3$ . **(a)**: No spontaneous adoption scenario  $\pi = 0$ : Three different values of the three-body spreading strength are shown ( $\lambda_2 = 0$ , red squares;  $\lambda_2 = 0.8$ , beige triangles;  $\lambda_2 = 2.5$ , blue circles), while varying the two-body spreading strength  $\lambda_1$ . Since the simulations agree with the mean field results,  $|m^*| = \rho^*$ . **(b) and (c)** depict the spontaneous adoption scenario with  $\pi = 0.05$ . Two different values of the three-body spreading strength are shown ( $\lambda_2 = 1.5$ , red squares;  $\lambda_2 = 3.9$ , blue circles). Other simulation parameters are  $r = 0.05$ ,  $N = 2000$ .

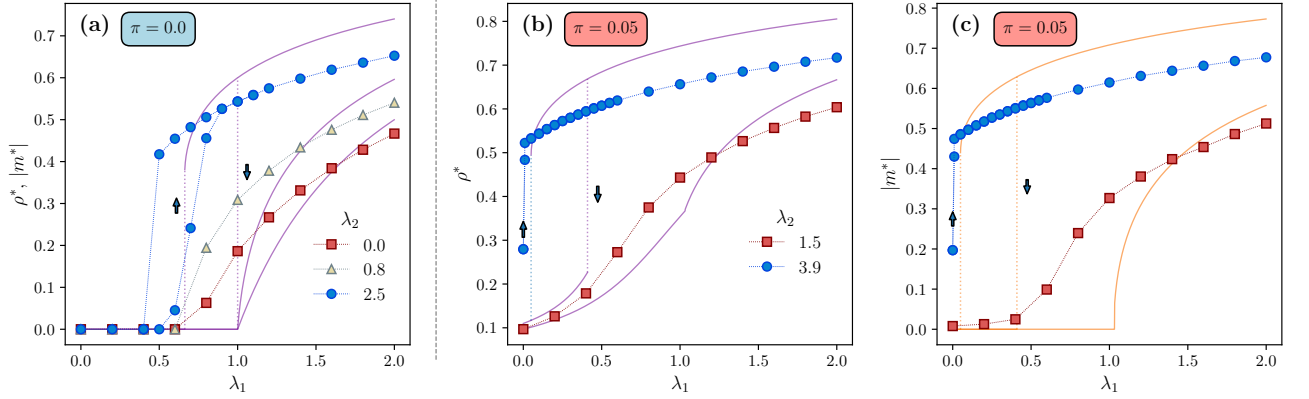

FIG. SF3: Simulations on a Simplicial Complex built from real data based on time-aggregated face-to-face interactions in a workplace. We use the same parameters as in the RSC simulations. **(a)**: The active population  $\rho^* = |m^*|$  for the no spontaneous adoption case  $\pi = 0$  and group recruitment strengths  $\lambda = 0.0, 0.8, 2.5$ . **(b) and (c)** show  $\rho^*$  and  $|m^*|$ , respectively, for the spontaneous adoption scenario with  $\pi = 0.05$  and group recruitment strengths  $\lambda = 1.5, 3.9$ . The system size of the simplicial complexes generated from the data is  $N = 1056$ , with average degree  $\langle k_1 \rangle = 25.9$  and average simplicial degree  $\langle k_2 \rangle = 7.0$ .
